# Supplementary material for: Parameter Optimization in Control Software using Statistical Fault Localization Techniques
Source: arXiv:1710.02073 source file (2017-10-09)
Supplement: Supplementary file 1 [file appendix.tex]

\section{Appendix}

\subsection{Syntax and Semantics of Signal Temporal Logic}

Most material appearing in this subsection is from \cite{DonzeM10}.
Let $\x$ denote a signal, \ie, a function from $\reals^{\ge 0}$ to
$\reals^n$.  Without loss of generality, atoms in STL formulas can be
be reduced to the form $f(x) \sim c$, where $f$ is a function from
$\reals^n$ to $\reals$, $\sim \in \setof{\geq,\leq,=}$, and $c \in
\reals$.  Temporal formulas are formed using temporal operators,
``always'' (denoted as $\alw$), ``eventually'' (denoted as $\ev$) and
``until'' (denoted as $\Until$) that can each be indexed by an interval
$\Intvl$.  An STL formula is written using the following grammar:
\begin{equation}
\label{eq:stl_syntax}
\begin{array}{l}
\Intvl := (a,b) \mid (a,b] \mid [a,b) \mid 
          [a,b] \mid [a,\infty) \mid (a,\infty) \\
\f :=      \true 
      \mid f(\x) \sim c
      \mid \neg\f \mid \f_{1} \wedge \f_{2} 
      \mid \alw_{\Intvl} \f 
      \mid \ev_{\Intvl} \f 
      \mid \f_{1}\, \Until_{\Intvl}\, \f_{2}~
\end{array}
\end{equation}
In the above grammar, $a,b \in \reals^{\ge 0}$, and $c \in \reals$.
The always ($\alw$) and eventually ($\ev$) operators are defined for
notational convenience, and are just special cases of the until
operator: \mbox{$\ev_{\Intvl}\varphi \triangleq \true\, \Until_\Intvl\,
\varphi$}, and \mbox{$\alw_{\Intvl}\varphi \triangleq \neg \ev_{\Intvl}
\neg \varphi$}.  We use the notation $(\x,t) \models \f$ to mean that
the suffix of the timed trace $\x$ beginning at time $t$ satisfies the
formula $\f$.  Formally, the semantics of an STL formula are defined
recursively as follows:

\vspace*{-4mm}
\begin{equation}
\label{eq:stl_semantics}
\begin{array}{lcl}
  (\x,t) \models f(\x) \sim c & \iff&
        \ \text{$f(\x(t)) \sim c$ is true} \\
  (\x,t) \models \neg \f &\iff&  
        (\x,t) \not\models \f \\
  (\x,t) \models \f_1 \wedge \f_2 &\iff& 
         (\x,t) \models \f_1\ \text{ and }  (\x,t) \models \f_2\\
  (\x,t) \models \alw_{\Intvl}(\f) & \iff & \forall t_1 \in t\oplus\Intvl: (\x,t_1) \models \f \\
  (\x,t) \models \ev_{\Intvl}(\f) & \iff & \exists t_1 \in t\oplus\Intvl: (\x,t_1) \models \f \\
  (\x,t) \models \f_1\ \Until_{\Intvl}\ \f_2 & \iff & \exists t_1\in t
  \oplus \Intvl: (\x,t_1) \models \f_2\ \wedge \\
  &      & \quad \forall t_2\in(t, t_1): (\x,t_2) \models \f_1
\end{array}
\end{equation}
We write $\x \models \f$ as a shorthand of $(\x,0) \models \f$.

\mypara{Quantitative Semantics for STL}
The \emph{quantitative semantics} of \STL are defined using a
real-valued function $\rob$ of a trace $\x$, a formula $\f$, and time
$t$ satisfying the following property:
\begin{equation}
  \rob(\f,\x,t) \geq 0\ \iff\ (\x,t) \models \f.
  \label{eq:qs_prop}
\end{equation}

Quantitative semantics capture the notion of \emph{robustness of
satisfaction} of $\f$ by a signal $\x$, \ie, whenever the absolute
value of $\rob(\f,\x,t)$ is large, a change in $\x$ is less likely to
affect the Boolean satisfaction (or violation) of $\f$ by $\x$.  In
\cite{DonzeM10}, different quantitative semantics for \STL have been
proposed. We recall the most commonly used semantics defined
inductively from the quantitative semantics for predicates and
inductive rules for each \STL operator.

Without loss of generality, an \STL predicate $\mu$ can be identified
to an inequality of the form $f(\x)\geq 0$ (the use of strict or non
strict inequalities is a matter of choice and other inequalities can
be trivially transformed into this form). From this form, a straightforward
quantitative semantics for predicate $\mu$ is defined as
\begin{equation}
\rob(\mu, \x,t)= f(\x(t)).
\label{eq:space}
\end{equation}

Then $\rob$ is defined inductively for every \STL formula using the
following rules:
 \begin{align}
   \label{eq:neg}
    \rob(\neg\f,\x,t)& =  -\rob(\f,\x,t) \\
    \label{eq:and}
    \rob(\f_1\wedge \f_2,\x,t)& =
    \min(\rob(\f_1,\x,t),\rob(\f_2,\x,t))\\
    \label{eq:until}
    \rob(\f_1\Until_I \f_2,\x,t)& = \displaystyle \sup_{t' \in t\oplus I} \big
    ( \min ( \rob(\f_2,\x,t'), \inf_{t''\in[t,t')} \rob(\f_1,\x,t'')\big)
 \end{align}
Then it can be shown \cite{DonzeM10} that $\rob$ satisfies
(\ref{eq:qs_prop}) and thus defines a quantitative semantics for
\STL. Additionally, by combining  (\ref{eq:until}),  and  \mbox{$\alw_{\Intvl}\varphi \triangleq
\neg \ev_{\Intvl} \neg \varphi$},  we get
\begin{align}
%\label{eq:ev}
%    \rob(\ev_I \f,\x,t)& =  \sup_{t' \in t+I} \rob(\f,\x,t') \\
\label{eq:alw}
    \rob(\alw_I \f,\x,t)& =  \inf_{t' \in t\oplus I} \rob(\f,\x,t')
\end{align}
For $\ev$, we get a similar expression using $\sup$ instead of $\inf$.

\subsection{The Intersection-Union model}

The intersection-union model in software fault localization defines the set of 
 suspicious statements   as consisting of  statements that are executed in \emph{every}
 failed run, but in \emph{none} of the successful runs~\cite{Pan92heuristicsfor}.
That is, the set of suspicious statements is given by
\[
\begin{array}{l}
\displaystyle\bigcap_{ z  \text{ s.t.} \score(z) <0} 
\set{\mathsf{s} \mid \mathsf{s}  \text{ executed by } z} \\
\qquad\qquad\qquad\qquad\qquad\qquad\setminus 
\displaystyle\bigcup_{ z  \text{ s.t.} \score(z) >0} 
\set{\mathsf{s} \mid \mathsf{s}  \text{ executed by } z} 
\end{array}
\]
This is a more stringent requirement for labelling statements as suspicious, compared
to the union model.

For the lookup map application, we modify this model by relaxing the
intersection,  and strengthening the set difference requirements  as follows.
For the intersection portion,
we consider the set (given a positive real number $r$):
\[
\Phi(r)  = \left\{ m \in M_F \ \left\lvert\ 
\begin{array}{l}
 \textbf{every } \text{ failed run } z \text{ accesses some } m_z\\
\text{such that }
 \ m_z\notin \ball(M_S, r_M) \text{ and}\\
 \dist(m, m_z) \leq r
\end{array}
\right.\!
\right\}.
\]
That is, $m\in \Phi(r)$ iff every failing run $z$ accesses some $m_z$ that is
(1)~at least $r_M$ distance away from $M_S$; and
(2)~at most $r$ distance away from $m$.
Thus, $m\in \Phi(r)$ iff every failing run $z$ accesses some index in
$M_F$ which is close-by
to $m$, and far away from $M_s$.

Note that if $r_2 < r_1$, then $\Phi(r_2) \subseteq \Phi(r_1)$, and that
$\Phi(0)$ equals the set
 \[
\Phi(0) = \left\{ m \in M_F \left\lvert
\begin{array}{l}
 \text{every } \text{ failed run } z \text{ accesses } m
\text{ with}\\
 m\notin  \ball(M_S, r_M)
\end{array}
\right.
\right\}.
\]
That is, 
\[
\Phi(0) = 
\begin{array}{c}
\left\{ m \in M_F \mid
\text{every } \text{ failed run } z \text{ accesses } m\right\}\\
\setminus \\
 \ball(M_S, r_M)
\end{array}
\]

We define the set of suspicious map indices  $\sus_{IU}$ as
\begin{equation}
\sus_{IU} = \Phi(r_M) \setminus \ball(M_S, r_M)
\end{equation}

Equivalently,  $\sus_{IU} =  \sus_U\cap  \Phi(r_M) $.

It can be shown that
\begin{equation}
\label{eq:IU}
\sus_{IU}=  \left\{ m \in \sus_U \ \left\lvert\ 
\begin{array}{l}
 \textbf{every } \text{ failed run } z \text{ accesses some } m_z\\
\text{such that }
 \ m_z\in \sus_U \text{ and}\\ \dist(m, m_z) \leq r_M
\end{array}
\right.\!
\right\}.
\end{equation}

The elements in   $\sus_{IU} $ are all highly suspicious, hence a ranking over
$\sus_{IU}$ is not necessary.
